# Supplementary material for: CRADL: Contrastive Representations for Unsupervised Anomaly Detection and Localization
Source: arXiv:2301.02126 source file (2023-01-05)
Supplement: Supplementary file 1 [file pixel_brats_2.tex]

\begin{tabular}{|lll|l|l|}
        \hline
                    &     &         &              AUPRC &              AUROC \\
        Pretext & Gen. Model & Score &                    &                    \\
        \hline
        VAE & GMM  1 Comp 
        % & nll &  0.0528$\pm$0.0073 &  0.6453$\pm$0.0138 \\
            % &     & nll+mask &  0.0931$\pm$0.0073 &  0.8537$\pm$0.0022 \\
            % &     & nll+mask+p5 &  0.1147$\pm$0.0103 &  0.8781$\pm$0.0026 \\
            % &
                & nll-grad &  0.1282$\pm$0.0123 &  0.8889$\pm$0.0023 \\
            % &     & nll+p5 &  0.0636$\pm$0.0087 &  0.7301$\pm$0.0159 \\
            % &     & nll+sm8 &  0.0797$\pm$0.0128 &  0.7727$\pm$0.0156 \\
            & GMM  2 Comp 
            % & nll &  0.0374$\pm$0.0051 &  0.5864$\pm$0.0147 \\
            % &     & nll+mask &  0.0853$\pm$0.0058 &   0.8495$\pm$0.002 \\
            % &     & nll+mask+p5 &  0.1004$\pm$0.0078 &  0.8712$\pm$0.0024 \\
            % &
                & nll-grad &  0.1095$\pm$0.0096 &  0.8808$\pm$0.0021 \\
            % &     & nll+p5 &  0.0401$\pm$0.0053 &  0.6457$\pm$0.0199 \\
            % &     & nll+sm8 &   0.048$\pm$0.0087 &  0.6865$\pm$0.0219 \\
            & GMM  4 Comp 
            % & nll &  0.0452$\pm$0.0078 &  0.6089$\pm$0.0147 \\
            % &     & nll+mask &  0.0941$\pm$0.0095 &  0.8555$\pm$0.0031 \\
            % &     & nll+mask+p5 &   0.1162$\pm$0.014 &   0.881$\pm$0.0041 \\
            % &
                & nll-grad &  0.1295$\pm$0.0173 &  0.8918$\pm$0.0038 \\
            % &     & nll+p5 &   0.0511$\pm$0.009 &  0.6831$\pm$0.0205 \\
            % &     & nll+sm8 &  0.0641$\pm$0.0142 &  0.7279$\pm$0.0231 \\
            & GMM  8 Comp 
            % & nll &  0.0468$\pm$0.0072 &   0.6145$\pm$0.012 \\
            % &     & nll+mask &   0.096$\pm$0.0076 &  0.8573$\pm$0.0023 \\
            % &     & nll+mask+p5 &  0.1201$\pm$0.0106 &   0.8838$\pm$0.003 \\
            % &     
                & nll-grad &   0.1345$\pm$0.013 &  0.8949$\pm$0.0026 \\
            % &     & nll+p5 &   0.0536$\pm$0.008 &  0.6921$\pm$0.0152 \\
            % &     & nll+sm8 &  0.0677$\pm$0.0131 &  0.7376$\pm$0.0182 \\
            % & INN 
            % % & nll &    0.032$\pm$0.007 &  0.5491$\pm$0.0393 \\
            % % &     & nll+mask &  0.0802$\pm$0.0075 &  0.8441$\pm$0.0061 \\
            % % &     & nll+mask+p5 &  0.0915$\pm$0.0106 &    0.86$\pm$0.0088 \\
            % % &     
            %     & nll-grad &   0.0978$\pm$0.012 &   0.8666$\pm$0.009 \\
            % % &     & nll+p5 &   0.033$\pm$0.0083 &  0.5789$\pm$0.0584 \\
            % % &     & nll+sm8 &  0.0382$\pm$0.0115 &   0.6122$\pm$0.063 \\
            \hline
            & VAE 
            % & combi &  0.1128$\pm$0.0107 &   0.8687$\pm$0.003 \\
            % &     
                & combi &  0.2269$\pm$0.0328 &  0.9198$\pm$0.0038 \\
            % &     & combi+sm &  0.1457$\pm$0.0207 &  0.8878$\pm$0.0043 \\
            % &     & kl-grad &  0.0329$\pm$0.0031 &  0.5673$\pm$0.0113 \\
            % &     & kl-grad+mask &  0.0694$\pm$0.0047 &  0.8306$\pm$0.0055 \\
            % &     & kl-grad+mask+p5 &  0.0736$\pm$0.0074 &  0.8384$\pm$0.0098 \\
            &     & kl-grad &  0.0772$\pm$0.0091 &   0.8446$\pm$0.011 \\
            % &     & kl-grad+mask+sm8 &  0.0751$\pm$0.0095 &  0.8379$\pm$0.0122 \\
            % &     & kl-grad+sm8 &    0.04$\pm$0.0055 &  0.6544$\pm$0.0234 \\
            % &     & rec &  0.1428$\pm$0.0028 &   0.892$\pm$0.0008 \\
            % &     & rec-grad &  0.0287$\pm$0.0008 &  0.4977$\pm$0.0016 \\
            % &     & rec+mask &  0.1437$\pm$0.0028 &  0.8935$\pm$0.0007 \\
            % &     & rec+mask+p5 &  0.2136$\pm$0.0035 &  0.9114$\pm$0.0007 \\
            &     & rec & \textbf{0.2976}$\pm$0.0035 &  \textbf{0.9248}$\pm$0.0006 \\
            % &     & rec+mask+sm8 &  0.2889$\pm$0.0039 &  0.9169$\pm$0.0006 \\
            % &     & rec+sm8 &  0.2827$\pm$0.0042 &  0.9161$\pm$0.0007 \\
            \hline
            \hline
ceVAE & GMM  1 Comp 
            % & nll &  0.0599$\pm$0.0221 &  0.6053$\pm$0.0333 \\
            % &     & nll+mask &  0.1468$\pm$0.0398 &  0.8692$\pm$0.0098 \\
            % &     & nll+mask+p5 &  0.2029$\pm$0.0653 &  0.9014$\pm$0.0137 \\
            % & 
                & nll-grad &  0.2343$\pm$0.0816 &  0.9129$\pm$0.0159 \\
            % &     & nll+p5 &  0.0729$\pm$0.0439 &   0.675$\pm$0.0615 \\
            % &     & nll+sm8 &  0.0972$\pm$0.0618 &  0.7224$\pm$0.0652 \\
            & GMM  2 Comp 
            % & nll &   0.034$\pm$0.0093 &  0.5483$\pm$0.0349 \\
            % &     & nll+mask &   0.1241$\pm$0.023 &  0.8669$\pm$0.0068 \\
            % &     & nll+mask+p5 &  0.1591$\pm$0.0353 &  0.8965$\pm$0.0084 \\
            % &     
                & nll-grad &   0.177$\pm$0.0426 &  0.9062$\pm$0.0097 \\
            % &     & nll+p5 &  0.0345$\pm$0.0122 &  0.5758$\pm$0.0546 \\
            % &     & nll+sm8 &  0.0421$\pm$0.0193 &   0.612$\pm$0.0564 \\
            & GMM  4 Comp 
            % & nll &  0.0331$\pm$0.0066 &  0.5522$\pm$0.0387 \\
            % &     & nll+mask &  0.1293$\pm$0.0115 &   0.869$\pm$0.0034 \\
            % &     & nll+mask+p5 &  0.1699$\pm$0.0157 &  0.9002$\pm$0.0035 \\
            % &     
                & nll-grad &  0.1906$\pm$0.0184 &   0.9105$\pm$0.004 \\
            % &     & nll+p5 &  0.0333$\pm$0.0084 &   0.584$\pm$0.0629 \\
            % &     & nll+sm8 &   0.0391$\pm$0.011 &  0.6219$\pm$0.0628 \\
            & GMM  8 Comp 
            % & nll &  0.0331$\pm$0.0049 &  0.5549$\pm$0.0322 \\
            % &     & nll+mask &  0.1379$\pm$0.0171 &  0.8712$\pm$0.0038 \\
            % &     & nll+mask+p5 &  0.1838$\pm$0.0276 &  0.9022$\pm$0.0047 \\
            % &     
                & nll-grad &   0.2068$\pm$0.033 &   0.9119$\pm$0.006 \\
            % &     & nll+p5 &  0.0331$\pm$0.0068 &  0.5849$\pm$0.0514 \\
            % &     & nll+sm8 &  0.0385$\pm$0.0084 &  0.6209$\pm$0.0497 \\
            % & INN 
            % % & nll &  0.0207$\pm$0.0027 &  0.4471$\pm$0.0485 \\
            % % &     & nll+mask &  0.0883$\pm$0.0093 &  0.8501$\pm$0.0068 \\
            % % &     & nll+mask+p5 &  0.1014$\pm$0.0154 &   0.8691$\pm$0.009 \\
            % % & 
            %     & nll-grad &  0.1072$\pm$0.0159 &  0.8756$\pm$0.0079 \\
            % % &     & nll+p5 &  0.0195$\pm$0.0028 &  0.4207$\pm$0.0641 \\
            % % &     & nll+sm8 &  0.0204$\pm$0.0032 &  0.4434$\pm$0.0642 \\
            \hline
            & VAE 
            % & combi &    0.281$\pm$0.027 &  0.8981$\pm$0.0042 \\
            % &
                & combi &   \textbf{0.483}$\pm$0.0299 &  \textbf{0.9482}$\pm$0.0032 \\
            % &     & combi+sm &  0.3868$\pm$0.0271 &  0.9218$\pm$0.0028 \\
            % &     & kl-grad &   0.1118$\pm$0.028 &  0.6516$\pm$0.0316 \\
            % &     & kl-grad+mask &  0.2017$\pm$0.0398 &  0.8812$\pm$0.0104 \\
            % &     & kl-grad+mask+p5 &  0.2962$\pm$0.0561 &   0.915$\pm$0.0142 \\
            &     & kl-grad &   0.3394$\pm$0.067 &  0.9252$\pm$0.0163 \\
            % &     & kl-grad+mask+sm8 &   0.341$\pm$0.0702 &  0.9253$\pm$0.0176 \\
            % &     & kl-grad+sm8 &  0.2134$\pm$0.0874 &   0.7801$\pm$0.059 \\
            % &     & rec &  0.1751$\pm$0.0325 &  0.8949$\pm$0.0065 \\
            % &     & rec-grad &   0.0646$\pm$0.028 &  0.5561$\pm$0.0333 \\
            % &     & rec+mask &  0.1765$\pm$0.0327 &  0.8985$\pm$0.0077 \\
            % &     & rec+mask+p5 &  0.3038$\pm$0.0428 &  0.9158$\pm$0.0074 \\
            &     & rec &  0.4073$\pm$0.0389 &  0.9269$\pm$0.0074 \\
            % &     & rec+mask+sm8 &  0.3887$\pm$0.0407 &  0.9172$\pm$0.0085 \\
            % &     & rec+sm8 &   0.3784$\pm$0.044 &  0.9161$\pm$0.0085 \\
            \hline
            \hline
SimCLR (ours) & GMM  1 Comp 
            % & nll &  0.1563$\pm$0.0213 &  0.8414$\pm$0.0107 \\
            % &     & nll+mask &   0.219$\pm$0.0245 &  0.9206$\pm$0.0045 \\
            % &     & nll+mask+p5 &  0.3006$\pm$0.0341 &  0.9334$\pm$0.0036 \\
            % &     
                & nll-grad &  0.3341$\pm$0.0402 &  0.9357$\pm$0.0035 \\
            % &     & nll+mask+sm8 &  0.2953$\pm$0.0391 &  0.9303$\pm$0.0039 \\
            % &     & nll+mask+sm8+p5 &  0.3051$\pm$0.0407 &  0.9312$\pm$0.0039 \\
            % &     & nll+p5 &  0.2044$\pm$0.0307 &  0.8738$\pm$0.0077 \\
            % &     & nll+sm8 &  0.2083$\pm$0.0333 &  0.8808$\pm$0.0073 \\
            % &     & nll+sm8+p5 &   0.214$\pm$0.0348 &   0.882$\pm$0.0073 \\
            & GMM  2 Comp 
            % & nll &  0.1827$\pm$0.0151 &   0.852$\pm$0.0058 \\
            % &     & nll+mask &  0.2519$\pm$0.0147 &  0.9274$\pm$0.0021 \\
            % &     & nll+mask+p5 &  0.3407$\pm$0.0155 &  0.9397$\pm$0.0009 \\
            % &
                & nll-grad &  \textbf{0.3802}$\pm$0.0163 &  \textbf{0.9418}$\pm$0.0009 \\
            % &     & nll+mask+sm8 &  0.3469$\pm$0.0182 &  0.9373$\pm$0.0009 \\
            % &     & nll+mask+sm8+p5 &  0.3582$\pm$0.0182 &  0.9381$\pm$0.0009 \\
            % &     & nll+p5 &  0.2421$\pm$0.0208 &  0.8812$\pm$0.0027 \\
            % &     & nll+sm8 &  0.2567$\pm$0.0224 &  0.8878$\pm$0.0024 \\
            % &     & nll+sm8+p5 &   0.2656$\pm$0.023 &  0.8888$\pm$0.0024 \\
            & GMM  4 Comp 
            % & nll &  0.1694$\pm$0.0131 &  0.8457$\pm$0.0066 \\
            % &     & nll+mask &  0.2324$\pm$0.0136 &  0.9239$\pm$0.0023 \\
            % &     & nll+mask+p5 &  0.3069$\pm$0.0145 &  0.9362$\pm$0.0014 \\
            % &     
                & nll-grad &  0.3383$\pm$0.0161 &  0.9384$\pm$0.0012 \\
            % &     & nll+mask+sm8 &   0.3106$\pm$0.018 &  0.9338$\pm$0.0014 \\
            % &     & nll+mask+sm8+p5 &  0.3198$\pm$0.0187 &  0.9346$\pm$0.0014 \\
            % &     & nll+p5 &  0.2199$\pm$0.0153 &  0.8758$\pm$0.0046 \\
            % &     & nll+sm8 &  0.2317$\pm$0.0187 &  0.8829$\pm$0.0042 \\
            % &     & nll+sm8+p5 &   0.239$\pm$0.0194 &   0.884$\pm$0.0041 \\
            & GMM  8 Comp 
            % & nll &  0.1388$\pm$0.0125 &  0.8303$\pm$0.0088 \\
            % &     & nll+mask &  0.1965$\pm$0.0138 &  0.9156$\pm$0.0037 \\
            % &     & nll+mask+p5 &   0.2609$\pm$0.017 &  0.9284$\pm$0.0023 \\
            % &     
                & nll-grad &  0.2908$\pm$0.0199 &  0.9309$\pm$0.0022 \\
            % &     & nll+mask+sm8 &  0.2632$\pm$0.0202 &  0.9257$\pm$0.0022 \\
            % &     & nll+mask+sm8+p5 &   0.2723$\pm$0.021 &  0.9267$\pm$0.0023 \\
            % &     & nll+p5 &  0.1791$\pm$0.0173 &  0.8626$\pm$0.0046 \\
            % &     & nll+sm8 &  0.1886$\pm$0.0191 &  0.8705$\pm$0.0039 \\
            % &     & nll+sm8+p5 &    0.1951$\pm$0.02 &   0.8718$\pm$0.004 \\
            % & INN 
            % % & nll &  0.0698$\pm$0.0095 &   0.6451$\pm$0.034 \\
            % % &     & nll+mask &   0.141$\pm$0.0126 &  0.8783$\pm$0.0081 \\
            % % &     & nll+mask+p5 &  0.1441$\pm$0.0117 &  0.8812$\pm$0.0076 \\
            % % &
            %     & nll-grad &  0.1362$\pm$0.0102 &  0.8736$\pm$0.0068 \\
            % % &     & nll+mask+sm8 &  0.1311$\pm$0.0106 &  0.8674$\pm$0.0074 \\
            % % &     & nll+mask+sm8+p5 &  0.1314$\pm$0.0105 &  0.8678$\pm$0.0074 \\
            % % &     & nll+p5 &  0.0706$\pm$0.0092 &  0.6476$\pm$0.0345 \\
            % % &     & nll+sm8 &  0.0707$\pm$0.0093 &  0.6515$\pm$0.0347 \\
            % % &     & nll+sm8+p5 &  0.0707$\pm$0.0093 &  0.6509$\pm$0.0348 \\    
        \hline
        GLOW & Normalizing Flow
        % & nll &     0.0147$\pm$0.0 &   0.237$\pm$0.0023 \\
        %   &           & nll+mask &  0.2299$\pm$0.0109 &  0.8725$\pm$0.0008 \\
        %   &           & nll+mask+p5 &  0.2889$\pm$0.0034 &  0.8899$\pm$0.0023 \\
        %   &
          & nll-grad &  0.3563$\pm$0.0023 &   0.9139$\pm$0.002 \\
        %   &           & nll+p5 &     0.0147$\pm$0.0 &  0.2285$\pm$0.0015 \\

\hline
        \end{tabular}
