# Supplementary material for: CRADL: Contrastive Representations for Unsupervised Anomaly Detection and Localization
Source: arXiv:2301.02126 source file (2023-01-05)
Supplement: Supplementary file 2 [file pixel_isles_2.tex]

% \begin{adjustbox}{totalheight=\textheight-2\baselineskip}
    \begin{tabular}{|lll|l|l|}
        \hline
                    &     &         &              AUPRC &              AUROC \\
        Pretext & Gen. Model & Score &                    &                    \\
        \hline
        VAE & GMM  1 Comp 
            % & nll &  0.0225$\pm$0.0012 &  0.6104$\pm$0.0086 \\
            % &     & nll+mask &  0.0401$\pm$0.0018 &  0.8264$\pm$0.0006 \\
            % &     & nll+mask+p5 &   0.0491$\pm$0.002 &  0.8501$\pm$0.0008 \\
            % & 
                & nll-grad &  0.0563$\pm$0.0033 &    0.86$\pm$0.0016 \\
            % &     & nll+p5 &  0.0255$\pm$0.0001 &   0.682$\pm$0.0121 \\
            % &     & nll+sm8 &  0.0336$\pm$0.0019 &  0.7242$\pm$0.0113 \\
            & GMM  2 Comp 
            % & nll &  0.0164$\pm$0.0002 &  0.5666$\pm$0.0073 \\
            % &     & nll+mask &  0.0367$\pm$0.0012 &  0.8228$\pm$0.0016 \\
            % &     & nll+mask+p5 &  0.0429$\pm$0.0016 &  0.8438$\pm$0.0027 \\
            % &   
                & nll-grad &  0.0471$\pm$0.0024 &  0.8523$\pm$0.0036 \\
            % &     & nll+p5 &  0.0169$\pm$0.0007 &  0.6136$\pm$0.0118 \\
            % &     & nll+sm8 &  0.0202$\pm$0.0001 &   0.6495$\pm$0.011 \\
            & GMM  4 Comp 
            % & nll &  0.0202$\pm$0.0008 &  0.5835$\pm$0.0093 \\
            % &     & nll+mask &  0.0403$\pm$0.0022 &  0.8263$\pm$0.0011 \\
            % &     & nll+mask+p5 &  0.0494$\pm$0.0036 &  0.8488$\pm$0.0024 \\
            % & 
                & nll-grad &  0.0562$\pm$0.0057 &  0.8578$\pm$0.0035 \\
            % &     & nll+p5 &   0.022$\pm$0.0007 &  0.6404$\pm$0.0162 \\
            % &     & nll+sm8 &  0.0287$\pm$0.0016 &  0.6799$\pm$0.0175 \\
            & GMM  8 Comp 
            % & nll &   0.021$\pm$0.0026 &  0.5885$\pm$0.0129 \\
            % &     & nll+mask &   0.0413$\pm$0.003 &  0.8282$\pm$0.0017 \\
            % &     & nll+mask+p5 &   0.0512$\pm$0.004 &  0.8515$\pm$0.0028 \\
            % & 
                & nll-grad &  0.0584$\pm$0.0058 &  0.8605$\pm$0.0028 \\
            % &     & nll+p5 &  0.0229$\pm$0.0021 &  0.6474$\pm$0.0199 \\
            % &     & nll+sm8 &    0.03$\pm$0.0043 &  0.6866$\pm$0.0237 \\
            % & INN 
            % % & nll &  0.0164$\pm$0.0015 &  0.5526$\pm$0.0221 \\
            % % &     & nll+mask &  0.0381$\pm$0.0033 &  0.8245$\pm$0.0025 \\
            % % &     & nll+mask+p5 &   0.0456$\pm$0.007 &  0.8443$\pm$0.0044 \\
            % % & 
            %     & nll-grad &  0.0498$\pm$0.0098 &  0.8516$\pm$0.0048 \\
            % % &     & nll+p5 &  0.0171$\pm$0.0017 &  0.5857$\pm$0.0332 \\
            % % &     & nll+sm8 &  0.0207$\pm$0.0029 &  0.6186$\pm$0.0375 \\
            \hline
            & VAE 
            % & combi &  0.0403$\pm$0.0034 &  0.8323$\pm$0.0039 \\
            % & 
                & combi &   \textbf{0.077}$\pm$0.0122 &  \textbf{0.8745}$\pm$0.0059 \\
            % &     & combi+sm &  0.0505$\pm$0.0071 &  0.8467$\pm$0.0049 \\
            % &     & kl-grad &  0.0163$\pm$0.0014 &   0.579$\pm$0.0101 \\
            % &     & kl-grad+mask &  0.0331$\pm$0.0022 &  0.8169$\pm$0.0043 \\
            % &     & kl-grad+mask+p5 &  0.0378$\pm$0.0036 &  0.8362$\pm$0.0076 \\
            &     & kl-grad &  0.0409$\pm$0.0047 &  0.8466$\pm$0.0081 \\
            % &     & kl-grad+mask+sm8 &   0.0403$\pm$0.005 &  0.8423$\pm$0.0091 \\
            % &     & kl-grad+sm8 &  0.0204$\pm$0.0028 &  0.6813$\pm$0.0183 \\
            % &     & rec &     0.0368$\pm$0.0 &  0.8338$\pm$0.0015 \\
            % &     & rec-grad &  0.0162$\pm$0.0009 &  0.5129$\pm$0.0016 \\
            % &     & rec+mask &     0.0369$\pm$0.0 &  0.8337$\pm$0.0014 \\
            % &     & rec+mask+p5 &  0.0441$\pm$0.0003 &  0.8461$\pm$0.0019 \\
            &       & rec &  0.0513$\pm$0.0001 &  0.8532$\pm$0.0023 \\
            % &     & rec+mask+sm8 &  0.0512$\pm$0.0003 &  0.8445$\pm$0.0023 \\
            % &     & rec+sm8 &  0.0511$\pm$0.0003 &  0.8441$\pm$0.0024 \\
            \hline
            \hline
ceVAE & GMM  1 Comp 
            % & nll &  0.0184$\pm$0.0047 &  0.5584$\pm$0.0364 \\
            % &     & nll+mask &  0.0437$\pm$0.0079 &  0.8285$\pm$0.0059 \\
            % &     & nll+mask+p5 &  0.0553$\pm$0.0137 &  0.8517$\pm$0.0075 \\
            % & 
                & nll-grad &  0.0618$\pm$0.0176 &    0.86$\pm$0.0089 \\
            % &     & nll+p5 &    0.0209$\pm$0.01 &  0.5987$\pm$0.0666 \\
            % &     & nll+sm8 &  0.0258$\pm$0.0136 &  0.6314$\pm$0.0685 \\
            & GMM  2 Comp 
            % & nll &  0.0113$\pm$0.0014 &  0.4915$\pm$0.0319 \\
            % &     & nll+mask &  0.0369$\pm$0.0048 &  0.8216$\pm$0.0051 \\
            % &     & nll+mask+p5 &  0.0425$\pm$0.0078 &   0.839$\pm$0.0061 \\
            % & 
                & nll-grad &  0.0449$\pm$0.0093 &  0.8445$\pm$0.0068 \\
            % &     & nll+p5 &  0.0108$\pm$0.0016 &  0.4842$\pm$0.0461 \\
            % &     & nll+sm8 &  0.0116$\pm$0.0021 &  0.5045$\pm$0.0458 \\
            & GMM  4 Comp 
            % & nll &  0.0116$\pm$0.0011 &  0.4961$\pm$0.0313 \\
            % &     & nll+mask &  0.0399$\pm$0.0063 &  0.8232$\pm$0.0049 \\
            % &     & nll+mask+p5 &  0.0476$\pm$0.0104 &  0.8404$\pm$0.0057 \\
            % & 
                & nll-grad &  0.0511$\pm$0.0123 &   0.8456$\pm$0.006 \\
            % &     & nll+p5 &   0.011$\pm$0.0014 &  0.4909$\pm$0.0468 \\
            % &     & nll+sm8 &  0.0119$\pm$0.0016 &  0.5118$\pm$0.0467 \\
            & GMM  8 Comp 
            % & nll &  0.0121$\pm$0.0013 &  0.5015$\pm$0.0298 \\
            % &     & nll+mask &   0.0445$\pm$0.004 &  0.8267$\pm$0.0036 \\
            % &     & nll+mask+p5 &   0.0558$\pm$0.007 &  0.8441$\pm$0.0047 \\
            % & 
                & nll-grad &  0.0612$\pm$0.0084 &  0.8488$\pm$0.0055 \\
            % &     & nll+p5 &  0.0116$\pm$0.0017 &  0.4966$\pm$0.0436 \\
            % &     & nll+sm8 &  0.0127$\pm$0.0019 &  0.5171$\pm$0.0415 \\
            % & INN 
            % % & nll &  0.0087$\pm$0.0006 &  0.4058$\pm$0.0394 \\
            % % &     & nll+mask &  0.0289$\pm$0.0002 &   0.805$\pm$0.0006 \\
            % % &     & nll+mask+p5 &    0.03$\pm$0.0006 &  0.8126$\pm$0.0011 \\
            % % &
            %      & nll-grad &  0.0304$\pm$0.0007 &  0.8157$\pm$0.0013 \\
            % % &     & nll+p5 &   0.008$\pm$0.0005 &  0.3584$\pm$0.0461 \\
            % % &     & nll+sm8 &  0.0081$\pm$0.0006 &    0.37$\pm$0.0482 \\
            \hline
            & VAE 
            % & combi &  0.0796$\pm$0.0057 &  0.8427$\pm$0.0014 \\
            % & 
                & combi &  \textbf{0.1451}$\pm$0.0125 &  \textbf{0.8794}$\pm$0.0022 \\
            % &     & combi+sm &  0.1208$\pm$0.0053 &  0.8578$\pm$0.0015 \\
            % &     & kl-grad &  0.0358$\pm$0.0092 &  0.6028$\pm$0.0519 \\
            % &     & kl-grad+mask &   0.0634$\pm$0.007 &  0.8418$\pm$0.0037 \\
            % &     & kl-grad+mask+p5 &  0.0923$\pm$0.0117 &  0.8694$\pm$0.0045 \\
            &     & kl-grad &  0.1085$\pm$0.0163 &  0.8785$\pm$0.0059 \\
            % &     & kl-grad+mask+sm8 &  0.1069$\pm$0.0133 &  0.8783$\pm$0.0065 \\
            % &     & kl-grad+sm8 &  0.0701$\pm$0.0292 &  0.7016$\pm$0.0938 \\
            % &     & rec &   0.0378$\pm$0.002 &   0.8351$\pm$0.004 \\
            % &     & rec-grad &  0.0204$\pm$0.0067 &  0.5052$\pm$0.0123 \\
            % &     & rec+mask &   0.038$\pm$0.0021 &  0.8372$\pm$0.0046 \\
            % &     & rec+mask+p5 &  0.0497$\pm$0.0027 &  0.8493$\pm$0.0049 \\
            &     & rec &  0.0653$\pm$0.0044 &   0.8544$\pm$0.005 \\
            % &     & rec+mask+sm8 &  0.0625$\pm$0.0055 &  0.8446$\pm$0.0059 \\
            % &     & rec+sm8 &  0.0622$\pm$0.0055 &   0.8436$\pm$0.006 \\
            \hline
            \hline
SimCLR (ours) & GMM  1 Comp 
            % & nll &  0.0825$\pm$0.0153 &  0.7703$\pm$0.0106 \\
            % &     & nll+mask &  0.1135$\pm$0.0197 &  0.8841$\pm$0.0044 \\
            % &     & nll+mask+p5 &   0.161$\pm$0.0326 &  0.8951$\pm$0.0035 \\
            % & 
                & nll-grad &  \textbf{0.1859}$\pm$0.0385 & \textbf{0.8977}$\pm$0.0033 \\
            % &     & nll+mask+sm8 &  0.1653$\pm$0.0372 &  0.8955$\pm$0.0034 \\
            % &     & nll+mask+sm8+p5 &  0.1716$\pm$0.0386 &  0.8958$\pm$0.0033 \\
            % &     & nll+p5 &  0.1152$\pm$0.0243 &   0.8045$\pm$0.008 \\
            % &     & nll+sm8 &  0.1248$\pm$0.0291 &  0.8191$\pm$0.0068 \\
            % &     & nll+sm8+p5 &  0.1302$\pm$0.0308 &  0.8198$\pm$0.0068 \\
            & GMM  2 Comp 
            % & nll &   0.0772$\pm$0.012 &   0.7681$\pm$0.009 \\
            % &     & nll+mask &  0.1057$\pm$0.0138 &  0.8829$\pm$0.0033 \\
            % &     & nll+mask+p5 &  0.1461$\pm$0.0195 &  0.8933$\pm$0.0028 \\
            % & 
                & nll-grad &    0.1653$\pm$0.02 &  0.8955$\pm$0.0029 \\
            % &     & nll+mask+sm8 &  0.1532$\pm$0.0207 &   0.8935$\pm$0.003 \\
            % &     & nll+mask+sm8+p5 &  0.1583$\pm$0.0206 &   0.8938$\pm$0.003 \\
            % &     & nll+p5 &  0.1066$\pm$0.0168 &  0.7999$\pm$0.0072 \\
            % &     & nll+sm8 &  0.1177$\pm$0.0188 &  0.8139$\pm$0.0069 \\
            % &     & nll+sm8+p5 &  0.1226$\pm$0.0193 &  0.8145$\pm$0.0069 \\
            & GMM  4 Comp 
            % & nll &  0.0715$\pm$0.0024 &  0.7647$\pm$0.0014 \\
            % &     & nll+mask &  0.0969$\pm$0.0031 &  0.8809$\pm$0.0018 \\
            % &     & nll+mask+p5 &  0.1291$\pm$0.0035 &  0.8912$\pm$0.0024 \\
            % &
                 & nll-grad &  0.1441$\pm$0.0024 &   0.8935$\pm$0.003 \\
            % &     & nll+mask+sm8 &  0.1357$\pm$0.0026 &  0.8915$\pm$0.0032 \\
            % &     & nll+mask+sm8+p5 &  0.1397$\pm$0.0023 &  0.8918$\pm$0.0033 \\
            % &     & nll+p5 &  0.0954$\pm$0.0023 &  0.7969$\pm$0.0034 \\
            % &     & nll+sm8 &  0.1052$\pm$0.0016 &  0.8114$\pm$0.0045 \\
            % &     & nll+sm8+p5 &  0.1091$\pm$0.0011 &  0.8121$\pm$0.0046 \\
            & GMM  8 Comp 
            % & nll &  0.0613$\pm$0.0076 &   0.758$\pm$0.0094 \\
            % &     & nll+mask &  0.0849$\pm$0.0088 &  0.8774$\pm$0.0036 \\
            % &     & nll+mask+p5 &   0.112$\pm$0.0131 &  0.8883$\pm$0.0023 \\
            % & 
                & nll-grad &  0.1257$\pm$0.0151 &  0.8906$\pm$0.0019 \\
            % &     & nll+mask+sm8 &  0.1172$\pm$0.0144 &  0.8884$\pm$0.0017 \\
            % &     & nll+mask+sm8+p5 &   0.121$\pm$0.0149 &  0.8888$\pm$0.0016 \\
            % &     & nll+p5 &  0.0806$\pm$0.0112 &  0.7918$\pm$0.0052 \\
            % &     & nll+sm8 &  0.0885$\pm$0.0125 &  0.8066$\pm$0.0036 \\
            % &     & nll+sm8+p5 &  0.0919$\pm$0.0132 &  0.8076$\pm$0.0035 \\
            % & INN 
            % % & nll &   0.0178$\pm$0.002 &  0.5431$\pm$0.0341 \\
            % % &     & nll+mask &  0.0395$\pm$0.0034 &  0.8234$\pm$0.0108 \\
            % % &     & nll+mask+p5 &  0.0407$\pm$0.0041 &   0.826$\pm$0.0136 \\
            % % & 
            %     & nll-grad &  0.0393$\pm$0.0044 &  0.8213$\pm$0.0153 \\
            % % &     & nll+mask+sm8 &    0.038$\pm$0.004 &  0.8153$\pm$0.0155 \\
            % % &     & nll+mask+sm8+p5 &  0.0381$\pm$0.0041 &  0.8154$\pm$0.0156 \\
            % % &     & nll+p5 &   0.018$\pm$0.0022 &  0.5439$\pm$0.0409 \\
            % % &     & nll+sm8 &  0.0182$\pm$0.0022 &  0.5519$\pm$0.0415 \\
            % % &     & nll+sm8+p5 &  0.0182$\pm$0.0022 &  0.5506$\pm$0.0419 \\
        \hline
        \hline
        GLOW & Normalizing Flow 
        % & nll &     0.0067$\pm$0.0 &   0.2147$\pm$0.003 \\
        %   &           & nll+mask &  0.0355$\pm$0.0007 &  0.8116$\pm$0.0023 \\
        %   &           & nll+mask+p5 &  0.0388$\pm$0.0017 &    0.82$\pm$0.0048 \\
        %   & 
          & nll-grad &  0.0443$\pm$0.0017 &  0.8307$\pm$0.0047 \\
        %   &           & nll+p5 &     0.0067$\pm$0.0 &  0.2016$\pm$0.0047 \\
         \hline
        \end{tabular}
    % \end{adjustbox}
